# Supplementary material for: A Theory of Second-Order Wireless Network Optimization and Its Application on AoI
Source: arXiv:2201.06486 source file (2022-01-17)
Supplement: Supplementary file 1 [file Appendix_A.tex]

\begin{appendices}
\section{The second-order statistics of a single ON/OFF Gilbert-Elliot channel} \label{Appendix: GE mean and variance}
This appendix aims to derive the mean $T\Bar{w}_i$ and variance $Tv_i$ for any consecutive slots $T$ of the Gilbert-Elliot model, and we follow the methods from Hablinger and Hohlfeld \cite{Gilbert1960GEmodel}. 

To achieve our goal, for any time $t$, we look at the following consecutive $T$ slots and obtain the number of slots that the channel $i$ is ON. 
For simplicity, we assume that the system has been running for a long time thus it is in the steady-state, and each sequence of $T$ slots has the same distribution. 
Then we number the slot from $1$ to $T$ in this sequence of $T$ slots, thus $W_i(t)$ is the indicator of $t$-th slot in this period.
We further define the $M_i(z,T) := \sum_k Pr\{\sum_{\tau = 1}^T W_i(\tau) = k\}z^k$ as the probability generating function for the number of ON channel in a sequence of $T$ slots.
By dividing the probability space, we obtain:
\begin{align}
    M_i(z,T) &= G_i(z,T) + B_i(z,T)\\
    G_i(z,T) &= \sum_{k=0}^T Pr\{\sum_{\tau = 1}^T W_i(\tau) = k, W_i(T) = 1\} z^k\\
    B_i(z,T) &= \sum_{k=0}^T Pr\{\sum_{\tau = 1}^T W_i(\tau) = k, W_i(T) = 0\} z^k,
\end{align}
where $G_i(z,T)$ and $B_i(z,T)$ are the generating function for the number of ON channel in a sequence of $T$ slots, leaving the Markov chain in the last state at state G and B, respectively.

We focus on $G_i(z,T)$, and continue dividing the probability space again to obtain two terms: 
\begin{align}
    &G_i(z,T) = L_1 + L_2 \\
    &L_1 = \sum_{k=0}^T Pr\{\sum_{\tau = 1}^T W_i(\tau) = k, W_i(T) = 1, \notag \\ &\qquad \qquad W_i(T-1) = 1\} z^k\\
    &L_2 = \sum_{k=0}^T Pr\{\sum_{\tau = 1}^T W_i(\tau) = k, W_i(T) = 1, \notag \\ &\qquad \qquad W_i(T-1) = 0\} z^k\\
\end{align}
For the first term $L_1$:
\begin{align}
    %1
    L_1 &=  \sum_{k=0}^T Pr\{\sum_{\tau = 1}^T W_i(\tau) = k, W_i(T) = 1, \notag \\ &\qquad  W_i(T-1) = 1\} z^k\\
    %2 k = k0 + k1
%    &= \sum_{k_0 + k_1=0}^T P\{\sum_{\tau = 1}^T W_i(\tau) = k_0 + k_1, W_i(T) = 1, \notag \\ &\qquad  W_i(T-1) = 1\} z^{k_0 + k_1}\\
    %3 bayes
    &= \sum_{k_0 + k_1=0}^T Pr\{\sum_{\tau = 1}^T W_i(\tau) = k_0 + k_1| W_i(T) = 1, \notag \\ &\qquad  W_i(T-1) = 1\} Pr\{W_i(T) = 1, W_i(T-1) = 1\} z^{k_0 + k_1}\\\label{f:G_T_derive_1}
    %4 using set and distributivity
    &= \sum_{k_0 + k_1=0}^T Pr\{\sum_{\tau = 1}^{T-1}W_i(\tau) = k_0 \bigcap W_i(T) = k_1 |W_i(T) = 1, \notag \\ &\qquad   W_i(T-1) = 1 \}Pr\{W_i(T) = 1, W_i(T-1) = 1\}z^{k_0 + k_1}\\  \label{f:G_T_derive_2}
    %5 divide k0 and k1 because condition
    &= \sum_{k_0 = 0}^{T-1}Pr\{\sum_{\tau = 1}^{T-1} W_i(\tau) = k_0|W_i(T) = 1, W_i(T-1) = 1\}z^{k_0}\notag \\ &\qquad \cdot \sum_{k_1 = 0}^1 Pr\{W_i(T) = k_1|W_i(T) = 1, W_i(T-1) = 1 \}\notag \\ &\qquad \cdot Pr\{W_i(T) = 1, W_i(T-1) = 1\} z^{k_1} \\ 
    %6 remove known part
%    &= \sum_{k_0 = 0}^{T-1}P\{\sum_{\tau = 1}^{T-1} W_i(\tau)= k_0| W_i(T-1) = 1\}z^{k_0}\notag \\ &\qquad \cdot P\{W_i(T) = 1, W_i(T-1) = 1\} z \\
    %7 bayes again
%    &= \sum_{k_0 = 0}^{T-1}P\{\sum_{\tau = 1}^{T-1} W_i(\tau)= k_0| W_i(T-1) = 1\}\notag \\ &\quad \cdot P\{W_i(T-1)=1\}z^{k_0}\cdot z\notag \\ &\qquad \cdot  P\{W_i(T)=1|W_i(T-1)=1\}\\
    %8 reverse-bayes
    &= \sum_{k_0 = 0}^{T-1}P\{\sum_{\tau = 1}^{T-1} W_i(\tau)= k_0, W_i(T-1) = 1\}z^{k_0}\notag \\ &\qquad \cdot z \cdot P\{W_i(T)=1|W_i(T-1)=1\}\\
    &=G_i(z,T-1)\cdot z\cdot (1-p_i) \label{f:G_T_term1},
\end{align} where $k_0$ and $k_1$ denotes the number of slots with ON channel in $[1,T-1]$ slots and the last slot $T$, respectively.
Moreover, from (\ref{f:G_T_derive_1}) to (\ref{f:G_T_derive_2}) is because events $\{\sum_{\tau = 1}^{T-1} W_i(\tau) = k_0|W_i(T) = 1, W_i(T-1) = 1\}$ and $P\{W_i(T) = k_1|W_i(T) = 1, W_i(T-1) = 1 \}$ are independent when given the condition. 

Since $L_1$ and $L_2$ are symmetric, we can apply the similar proof and obtain:
\begin{align}
    L_2 = B_i(z,T-1) r_i \label{f:G_T_term2}.
\end{align}
Consequently, 
\begin{align}
    G_i(z,T) =G_i(z,T-1)(1-p_i)z + B_i(z,T-1) r_i\label{f:G equation} 
\end{align}

Again, $G_i(z,T)$ and $B_i(z,T)$ are also symmetric, thus $B_i(z,T)$ can also be obtained as: 
\begin{align}
    B_i(z,T) = G_i(z,T-1)p_i z +  B_i(z,T-1) (1-r_i)\label{f:B equation}
\end{align}

Recall we assume the system is in steady-state,  the above expressions are initialized with starting point:
\begin{align}
    G_i(z,0) = \frac{r_i}{p_i + r_i},\quad B_i(z,0) = \frac{p_i}{p_i+r_i} 
\end{align}

Given the generating function, the $k$-th moment can be obtained by taking the $k$-th derivative. 
Further, the second-order statistics can be obtained by the first and second derivatives of the generating function when setting $z = 1$.
Specifically, we have the mean $T \Bar{w}_i$ and variance $T v_i$ are given by: 
\begin{align}
    T \Bar{w}_i &= G'_i (1,T) +  B'_i (1,T)\\
    T v_i &= G''_i (1,T) +  B''_i (1,T) + T \Bar{w}_i - (T \Bar{w}_i)^2.
\end{align}

The mean $T \Bar{w}_i$ leads to the $T$ times the steady-state fraction of ON channel:
\begin{align}
    T \Bar{w}_i = T\frac{r_i}{p_i + r_i}
\end{align}

For the variance, it turns out to be an iterative expression due to the symmetry of two states:
\begin{align}
    &G''_i (1,T) +  B''_i (1,T) \notag \\ &\quad = G''_i (1,T-1) +  B''_i (1,T-1) + 2 G'_i (1,T) \notag \\
    &\quad = 2 \sum_{\tau = 1}^T G'_i (1,\tau)
\end{align}
Eventually, we obtain the explicit expression for the variance:
\begin{align}
    Tv_i &= \frac{2Tr_i^2+Tp_ir_i}{(p_i+r_i)^2}  + \frac{2p_ir_i(1-p_i-r_i)}{(p_i+r_i)^3}T \notag \\ &\qquad- \frac{2p_ir_i((1-p_i-r_i)^2-(1-p_i-r_i)^{T+2})}{(p_i+r_i)^4}.
\end{align}

~\\

\section{The Performance Deviation of the LVWD Policy under the I.I.D system}\label{Appendix: iid positive recurrent}
Recall for the I.I.D system, we have:
\begin{align}
    W_i(t) = \begin{cases}
    &1,\quad  w.p. \quad q_i\\
    &0, \quad w.p. \quad 1-q_i
    \end{cases}
\end{align}
Under the VWD policy, the system sorts all flows as $v_1d_1(t)\geq v_2d_2(t) \geq \dots\geq v_Nd_N(t)$ and selects the flow with largest $v_id_i(t)$ among all ON flows. 
Hence, suppose $r_t$ is the flow that is selected at time $t$ under VWD, then it must satisfy two conditions: first, flow $r_t$ is ON; Second, all flows with smaller index numbers are OFF. 
It leads to the probability of flow $r_t$ that can be scheduled is denoted by $\Tilde{q}_{r_t} := Pr\{(\bigcap_{i=1}^{r_t-1} W_i(t) = 0)\bigcap W_i(t)=1\} = q_{r_t} \prod_{i=1}^{r_t-1}q_i$ . 
Therefore, we have $\Delta X_{r_t}(t) = 1$ with probability $\Tilde{q}_{r_t}$, and $\Delta X_{r_t}(t) = 0$ with probability $1-\Tilde{q}_{r_t}$. 
Then we have: $E[\Delta X_{r_t}(t)] =\Tilde{q}_{r_t}$.
For all other flows $i \neq r_t$, $\Delta X_i(t) = 0$. The above analysis gives:
\begin{align}
    \sum_{i=1}^N E[\Delta X_i(t)] = \sum_{i=1}^N  \Tilde{q}_{i}
    %&= p_1 + (1-p_1)p_2 + \dots +  p_{N} \prod_{i=1}^{N-1}p_i \\
    = \mu_{\{1,2,\dots, N\}}, 
\end{align}
and, for all $j < N$, 
\begin{align}
    \sum_{i=1}^j E[\Delta X_i(t)]  = \sum_{i=1}^j  \Tilde{q}_{i}
   %&= p_1 + (1-p_1)p_2 + \dots +  p_{j} \prod_{i=1}^{j-1}p_i \\
    = \mu_{\{1,2,\dots, j\}}.
\end{align} 

Recall (\ref{f:c min}) and (\ref{f:formal equa xbar}), we further derive conclusions for deficit increment: 
\begin{align}
       &E[\sum_{i=1}^N \Delta d_i(t)] = E[\sum_{i=1}^N \Bar{X}_i^* - \sum_{i=1}^N\Delta X_i(t)] = 0 \\
       &E[\sum_{i=1}^j \Delta d_i(t)] = E[\sum_{i=1}^j \Bar{X}_i^* - \sum_{i=1}^j\Delta X_i(t)] \leq -C_{min}
\end{align}
We also have:
\begin{align}
    E[\Delta D(t)] = 0.
\end{align}

Now we are ready to continue our deviration for (\ref{f:lya drift one slot}):
\begin{align}
    %&\Delta (L(t)) := E[L(t+1) - L(t)|H^t]\notag \\ 
    %&= E[\frac{1}{2} \sum_{i=1}^N \frac{1}{v_i}(v_id_i(t+1)-D(t+1))^2 \notag \\ &\quad - \frac{1}{2} \sum_{i=1}^N \frac{1}{v_i}(v_id_i(t)-D(t))^2|H^t]\\
    %&= E[\frac{1}{2} \sum_{i=1}^N \frac{1}{v_i} (v_id_i(t)-D(t)+v_i\Delta d_i(t)-\Delta D(t))^2 \notag \\ &\quad -  \frac{1}{2} \sum_{i=1}^N \frac{1}{v_i}(v_id_i(t)-D(t))^2|H^t]\\
    %&= E[\frac{1}{2} \sum_{i=1}^N \frac{1}{v_i} (v_i\Delta d_i(t) - \Delta D(t))^2 \notag \\ &\quad + \sum_{i=1}^N \frac{1}{v_i} (v_id_i(t)-D(t))\cdot(v_i\Delta d_i(t) - \Delta D(t))|H^t]\\
    &\Delta (L(t)) \leq B + E[\sum_{i=1}^N  g_i(t) y_i(t)|H^t]\notag \\
    %&= B + E[\sum_{i=1}^N \frac{1}{v_i} (v_id_i(t)-D(t))\cdot(v_i\Delta d_i(t) - \Delta D(t))]\\
    %&= B + E[\sum_{i=1}^N (v_id_i(t)-D(t))\Delta d_i(t)]\\
    %&= B + E[\sum_{i=1}^N v_id_i(t)\Delta d_i(t)]\\
    %&= B + E[\sum_{i=1}^N v_id_i(t)(\Bar{X}_i^* - \Delta X_i(t))]\\
    %&= B + E[\sum_{i=1}^N v_id_i(t)\Bar{X}_i^*] - E[\sum_{i=1}^N v_id_i(t)\Delta X_i(t))]\\
    %&=B + E[\sum_{i=1}^N v_id_i(t)\Bar{X}_i^*] - v_{r_t}d_{r_t}(t)
    &= B + E[[g_1(t)-g_2(t)]y_1(t) + [g_2(t)-g_3(t)][y_1(t)+y_2(t)]]\notag \\&\quad  + \dots + [g_{N-1}(t) - g_N(t)]\sum_{i=1}^{N-1} y_i(t) + g_N(t)\sum_{i=1}^N y_i(t)\\
    &=  -C_{min} [g_1(t)-g_N(t)] + B,
\end{align} since $y_i(t) :=\frac{1}{v_i} (v_i\Delta d_i(t) - \Delta D(t))$ ,$\sum_{i=1}^j E[y_i(t)] =\sum_{i=1}^j E[\Delta d_i(t)] $, and $\sum_{i=1}^N E[y_i(t)] =\sum_{i=1}^N E[\Delta d_i(t)] $.

Recall that $g_1(t) \geq g_2(t) \geq \dots \geq g_N(t)$. 
Hence $[g_1(t) - g_N(t)] \geq  |d_i(t) - D(t)| \geq 0$ for all $i$. 
For some $i$, if we have $|d_i(t) - D(t)|> \frac{B}{C_{min}}+1$, then $\Delta (L(t)) < -C_{min}$; Otherwise, we have $\Delta (L(t)) \geq B$.
By the Foster-Lyapunov theorem, the Markov process with state vector $\{v_id_i(t) - D(t)\}$ is positive recurrent.

\end{appendices}
